# Supplementary material for: Towards Flexible Intensity Control of Resonantly Scattered $\gamma$-Rays Using Multi-Frequency Vibrating Resonant Absorber
Source: arXiv:2410.05277 source file (2025-03-13)
Supplement: Supplementary file 1 [file Supplemental_Material_rev1.pdf]

# Towards Flexible Intensity Control of Resonantly Scattered $\gamma$-Rays Using Multi-Frequency Vibrating Resonant Absorber

## SUPPLEMENTAL MATERIAL

Aleš Stejskal, Vlastimil Vrba, and Vít Procházka
*Department of Experimental Physics, Faculty of Science, Palacký University Olomouc, 17. listopadu 1192/12, 779 00 Olomouc, Czech Republic*

This supplemental material contains a description of the numerical calculation of $\gamma$-ray intensity passing through a multi-frequency vibrating absorber. The calculations are also simplified to optimize the computation time by avoiding negligible expressions. Furthermore, details of the experimental setup, mainly the piezo-transducer, are provided. Next, the procedure of measuring the frequency response function of the piezo-transducer is described. Finally, the normalization of experimentally measured $\gamma$-ray intensity is specified so it can be compared with simulations.

### I. NUMERICAL CALCULATIONS OF $\gamma$-RAY INTENSITY PASSING THROUGH A MULTI-FREQUENCY VIBRATING ABSORBER

Coherent control of $\gamma$-photons emitted by a radioactive source through ultrasound vibrations of an absorber can be described using a semi-classical approach. In the laboratory reference frame, the $\gamma$-photon field incident on the vibrating absorber can be represented as a classical quasi-monochromatic wave

$$E(z,t) = E_0\theta\left(t - t_0 - \frac{z}{c}\right)\exp\left[-\left(i\omega_r + \frac{\Gamma}{2}\right)\left(t - t_0 - \frac{z}{c}\right) + i\varphi_0\right], \tag{S1}$$

where $E_0$ is the wave amplitude, $\omega_r$ is the resonant frequency, $\theta$ is the Heaviside step function, $\Gamma$ is the inverse of the excited state lifetime, $t_0$ is the origin time of the excited state, $c$ is the speed of light in vacuum, $i$ is the imaginary unit, $\varphi_0$ is an initial random phase, and $z$ is the absorber coordinate along the $\gamma$-photon propagation direction. Note that the phase $\varphi_0$ can be neglected, because it plays role only in the multiple photon interference. Further, we consider general periodic uniform absorber motion $z(t)$ expressed by the Fourier series

$$z(t) = z_0 + Az'(t) = z_0 + A\sum_{k=1}^{K} a_k \sin\left(2\pi k f t + \phi_k\right), \tag{S2}$$

where $z_0$ is the rest distance between the absorber and the radioactive source, $A$ is the amplitude of the absorber motion, $z'(t)$ is the normalized shape of the absorber motion profile ($\max|z'(t)| = 1$), $a_k$ and $\phi_k$ are the normalized Fourier coefficients, $K$ specifies the number of harmonics used to realize the motion ($a_k = 0$ for $k > K$), and $f$ is a fundamental frequency. The amplitude $A$ can be rewritten using the dimensionless modulation parameter $p$, which is related to the $\gamma$-photon wavelength $\lambda$ as $p = 2\pi A/\lambda$, yielding

$$z(t) = z_0 + \frac{pc}{\omega_r}z'(t). \tag{S3}$$

Note that the distance between the absorber and radioactive source also changes due to constant velocity of Doppler energy modulation. However, this motion manifests only as a shift of $\gamma$-photon energy $\Delta$ (energy detuning from the resonance). Impact of the Doppler modulation on the scattering process can be neglected as it is over five orders of magnitude slower compared to absorber vibrations. By inserting Eq. S3 into Eq. S1 the modulated photon field can be expressed as:

$$E(z,t) = E_0\theta\left(t - t_0 - \frac{z_0}{c} - \frac{pz'(t)}{\omega_r}\right)\exp\left[-\left(i\omega_r + \frac{\Gamma}{2}\right)\left(t - t_0 - \frac{z_0}{c} - \frac{pz'(t)}{\omega_r}\right)\right]. \tag{S4}$$

To calculate the normalized $\gamma$-ray intensity, the photon field is scaled to unit area by setting $E_0 = \sqrt{\Gamma}$. Further, some expressions in Eq. S4 may by neglected to optimize calculations. Specifically, in the argument of Heaviside function $z_0/c$ can be neglected as it introduces only constant time shift of maximally a few nanoseconds and $[pz'(t)]/\omega_r$ may be neglected since it is over nine orders of magnitude lower than $t_0$, which is on the order of nanoseconds (for the

first excited state of the $^{57}$Fe $w_s \approx 2.2 \times 10^{19}$ rad/s). In the exponent, only $z_0/c$ can be neglected, since it introduces unimportant phase shift. Thus, the photon field for the calculations has the form

$$E(z,t) = \sqrt{\Gamma}\theta\,(t-t_0) \times \exp\left[-\left(i\omega_r + \frac{\Gamma}{2}\right)\left(t - t_0 - \frac{pz'(t)}{\omega_r}\right)\right]. \tag{S5}$$

The photon interacts with the absorber, which can be described in the energy domain by the complex absorption function $\tilde{S}(\omega)$. The nature of nuclear absorption lines is Lorentzian, so the singlet absorber can be described as follows:

$$\tilde{S}(\omega) = \frac{i\frac{\Gamma}{2}}{(\omega - \omega_\mathrm{s} - \delta) + i\frac{\Gamma}{2}}\,, \tag{S6}$$

where $\delta$ is the shift of the centre of the absorption line with respect to the source emission line. For the purposes of the experiments, we consider a magnetically split absorber because it is necessary to take into account even small effective magnetic fields ($< 1\,\mathrm{T}$). The absorption function is then given by the sum of six Lorentzians

$$\tilde{S}(\omega) = \sum_{m=1}^{6} b_\mathrm{m} \frac{i\frac{\Gamma}{2}}{(\omega - \omega_r - \delta - \Delta\omega_\mathrm{m}) + i\frac{\Gamma}{2}}\,, \tag{S7}$$

where $b_m = \frac{3}{12}, \frac{2}{12}, \frac{1}{12}, \frac{1}{12}, \frac{2}{12}, \frac{3}{12}$ for $m = 1, \ldots, 6$ are the normalized amplitudes of the sextet lines and the term $\omega_0 - \delta - \Delta\omega_\mathrm{m}$ defines their positions. The expression $\Delta\omega_\mathrm{m}$ depends on the hyperfine magnetic field $B_\mathrm{hf}$ at the absorber nuclei and follows the equation

$$\Delta\omega_\mathrm{m} = (g_\mathrm{g} m_\mathrm{g} - g_\mathrm{e} m_\mathrm{e})\,\mu_\mathrm{n} B_\mathrm{hf}, \tag{S8}$$

where $\mu_\mathrm{n} = 31.5245\,\mathrm{neV/T}$ is nuclear magneton, $g_\mathrm{g}$ and $g_\mathrm{e}$ are g-factors of the ground and excited state and $m_\mathrm{g}$ and $m_\mathrm{e}$ are their magnetic numbers, which must satisfy the selection rules $m_\mathrm{e} - m_\mathrm{g} = 0, \pm 1$. Specifically for $^{57}$Fe, these values are: $g_\mathrm{g} = 0.18125$, $g_\mathrm{e} = -0.10348$, $m_\mathrm{e} = -3/2, -1/2, +1/2, 3/2$, and $m_\mathrm{g} = -1/2, +1/2$.

The procedure of the numerical calculation of the $\gamma$-ray intensity is similar to the analytical derivation of transmission Mössbauer spectrum. The incident photon field $E(z,t)$ is transformed into the energy domain by the fast Fourier transform (FFT). Subsequently, the photon field after the scattering process $E_\mathrm{out}(\omega)$ is obtained by multiplying the energy domain of the photon field $\tilde{E}(\omega)$ and the absorption function $\tilde{S}(\omega)$ according to the equation

$$\tilde{E}_\mathrm{out}(\omega) = \tilde{E}(\omega)\mathrm{exp}\left(-\frac{T_\mathrm{a}}{2}\tilde{S}(\omega)\right)\,. \tag{S9}$$

The quantity $T_\mathrm{a}$ is the optical (effective) thickness of the absorber and is defined by the relation

$$T_\mathrm{a} = \sigma_0 \eta f_\mathrm{LM} d\,, \tag{S10}$$

where $\sigma_0$ ($2.56 \times 10^{-6}$ b/atom for $^{57}$Fe [22]) is the differential cross section of the nuclear resonant interaction, $\eta$ is the number of Mössbauer nuclei per unit volume, $f_\mathrm{LM}$ is a Lamb-Mössbauer factor determining the probability of recoilless interaction and $d$ is the physical thickness of the absorber.

The scattered field $\tilde{E}_\mathrm{out}(\omega)$ is subsequently transformed back into the time domain by inverse FFT, giving $E_\mathrm{out}(t)$. The experimentally measurable radiation intensity $I_\mathrm{out}(t)$ is then obtained as a modulus of the output photon field $E_\mathrm{out}(t)$ using the complex conjugate

$$I_\mathrm{out}(t) = E_\mathrm{out}(t)E^*_\mathrm{out}(t) = \mid E_\mathrm{out}(t) \mid^2\ . \tag{S11}$$

However, this is the intensity calculated only for a specific value of $t_0$. Since we are interested in the radiation intensity measured relative to the absorber motion profile rather than the origin of the excited state, the random nature of the radioactive decay must be considered. Deexcitation at time $t_0$ after the excited state origin has an exponential distribution, but the excited state originates at random times, so the resultant distribution of the parameter $t_0$ is uniform. For that reason, the resulting normalized $\gamma$-ray intensity is given by the integral

$$I(t) = \int_{-\infty}^{\infty} I_\mathrm{out}(t, t_0)\, dt_0\,. \tag{S12}$$

The Python script "multifrequency_gamma_control.py" performing the above described calculations is enclosed with this supplemental material to reproduce the simulations presented in the Letter.

## II. EXPERIMENTAL SETUP DETAILS

The experimental setup was controlled by OLTWINS Mössbauer spectrometer [23], which allows besides the standard Mössbauer experiments also the measurement of delayed coincidence experiments and time-differential Mössbauer spectra. This allows sorting the detected 14.4 keV photons not only according to the Doppler energy modulation but also by the time of flight from the starting event. In addition, the spectrometer enables acquiring two time histograms simultaneously for different phases of Doppler energy modulation. Typically the first histogram is measured for positive energy (velocity) and the second for negative one, see Fig. 10 in Ref. [23].

When measuring the $\gamma$-ray intensity, the time measurements were started by a signal from the arbitrary function generator Siglent SDG2042, marking the beginning of the period of the signal driving the absorber motion, and stopped by the detection of the first 14.4 keV photon. The time intervals were measured with 2 ns time resolution determining also the width of histogram time bins. Nevertheless, the time resolution of the entire apparatus was 12 ns FWHM, see Section III.

The piezo transducer used to move the absorber was assembled from a 28 $\mu$m thick polyvinylidene fluoride (PVDF) piezoelectric foil (model LDT0-28K by Measurement Specialties, Inc.), 2 mm thick plexiglass backing, and stainless steel foil absorber [type 304, production No. 41580, with a natural abundance of $^{57}$Fe (2.119 %) from Alfa Aesar, now available from Fischer Scientific]. The piezoelectric foil was stuck to the plexiglass backing and the absorber was stuck to the piezoelectric foil by epoxy glue. The cross section of the piezo transducer and the specific piece used in the experiments are shown in Fig. S1. A lead mask used for collimation of $\gamma$-rays had the square hole with dimensions 6×6 mm and was mounted near the piezo transducer at a distance of 10 cm from the radioactive source.

The voltage waveform driving the piezo transducer was generated by the second channel of the aforementioned generator SDG2042. Required voltage waveforms were loaded into the generator via EasyWave application, which allows the waveform to be defined by an equation. The signal from the generator was amplified by a purpose-built RF amplifier based on the operational amplifier THS3491. It has 50 Ω input termination, a constant gain of 5, a low output impedance of about 9 Ω, and higher maximum output voltage of ±15 V compared to the generator.

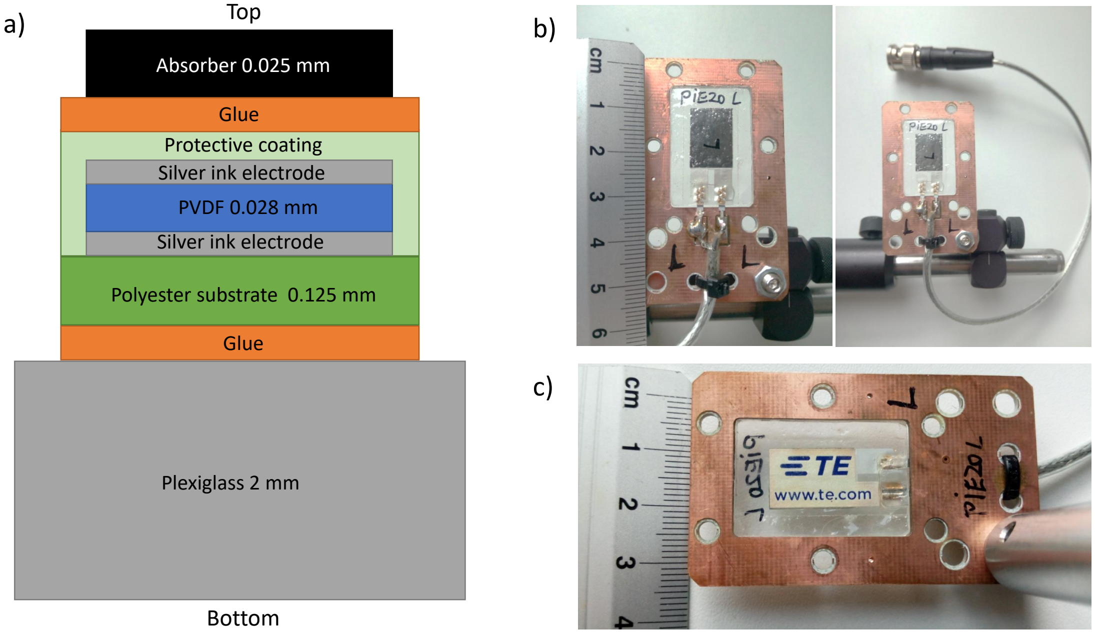


FIG. S1: Cross section of the piezo transducer (a), view of the piezo transducer from top (b), and bottom (c).

## III. MEASUREMENT OF PIEZO TRANSDUCER FREQUENCY RESPONSE.

The response function of the piezo transducer, i.e., the relationship between the voltage set on the arbitrary function generator and the motion of the absorber, was measured point by point for each specific frequency and amplitude of sinusoidal driving voltage. For each pair of these values, amplitude $A$ and phase $\phi$ of the absorber motion were determined by fitting the radiation intensity. See the example of the measurements in Fig. S2 (measured on a different piezo-element than the final results) presenting the dependence of the $\gamma$-ray intensity on the amplitude of the sinusoidal driving voltage. Experimental data were fitted using the function $I_{\rm exp}(t)$, which we defined by a convolution of $\gamma$-ray intensity scaled to data $I_s(t)$ and the Gaussian time resolution $G(t)$ of the apparatus

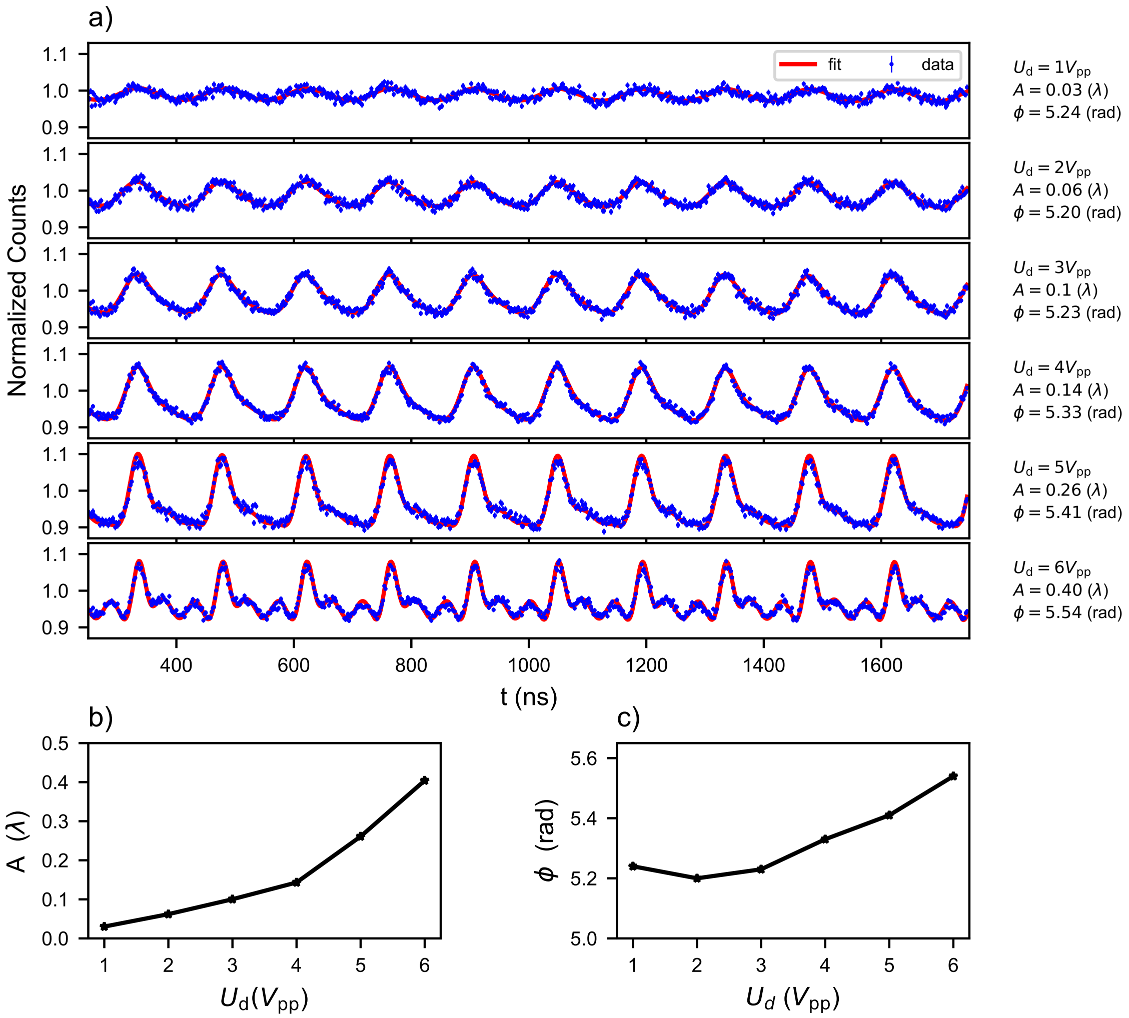


FIG. S2: Determination of amplitude $A$ and phase $\phi$ of the sinusoidal absorber motion from fitting the $\gamma$-ray intensity waveforms (a). Measurements are performed for different amplitudes of driving voltage $U_{\rm d}$ at frequency 7 MHz. The experimental data are normalized by fitted number of counts $N$ The phase shift $\phi$ was referenced to the zero phase of driving voltage. Parts (b) and (c) show dependence of vibrations amplitude and phase on driving voltage amplitude.

$$I_{\rm exp}(t) = I_s(t) * G(t)\,, \tag{S13}$$

where

$$G(t) = \frac{1}{\sqrt{2\pi}\sigma_{\rm t}} \exp\left[-\left(\frac{t}{\sqrt{2}\sigma_{\rm t}}\right)^2\right], \tag{S14}$$

which includes parameter $\sigma_t$ related to the FWHM of the apparatus time resolution as FWHM $\approx 2.35\sigma_{\rm t}$. Function $I_s(t)$ is defined as

$$I_s(t) = \left(\frac{I(t) + A_{\rm bcg}}{1 + A_{\rm bcg}}\right) N \exp\left(-\frac{t}{C_{\rm b}}\right) , \tag{S15}$$

where $I(t)$ is calculated normalized $\gamma$-ray intensity defined by Eq. S12 in Section I, $A_{\rm bcg}$ is non-resonant background (including detector noise), $N$ is number of counts, and parameter $C_{\rm b}$ describes an exponential decrease in countrate of longer time intervals which is caused by electronics. The processing unit detects only the first 14.4 keV photon after the start pulse and ignores all subsequent photons. For that reason the probability of detecting a particle decreases the longer time elapsed from the start pulse. The other parameters: $A$, $\phi$, $f$, $\Delta$, $T_{\rm a}$, and $B_{\rm hf}$, are included in the $I(t)$.

To obtain sufficiently precise values of $A$ and $\phi$, it was necessary to fix the absorber parameters $T_{\rm a}$, $B_{\rm hf}$, the apparatus time resolution $\sigma_t$, and the non-resonant background $A_{\rm bcg}$. Primarily, the last two parameters are undesirably correlated with the absorber motion amplitude $A$. If they are not fixed, the amplitude may diverge from real value by even over 20 %.

The optical thickness $T_{\rm a} = 7.6 \pm 0.3$ and the hyperfine magnetic field of the absorber $B_{\rm hf} = 0.58 \pm 0.02$ T were determined by means of Mössbauer resonant spectroscopy [22]. The non-resonant background parameter $A_{\rm bcg}$ was calculated using the following equation

$$A_{\rm bcg} = \frac{a_{\rm n}}{a_{\rm e}} - 1 , \tag{S16}$$

where $a_{\rm n}$ is the amplitude of normalized nuclear absorption peak of the resonant photons and $a_{\rm e}$ is the amplitude of the absorption peak in the transmission Mössbauer spectrum (usually called Mössbauer effect) of the absorber at rest (no vibrations applied). $a_{\rm e}$ was calculated from the transmission spectrum as

$$a_{\rm e} = \frac{N_{\rm out} - N_{\rm r}}{N_{\rm out}} , \tag{S17}$$

where $N_{\rm out}$ is the number of counts out of the resonance and $N_{\rm r}$ represents number of counts at the resonance, see Fig. S3(a). $a_{\rm n}$ was computed using aforementioned numerical calculations of normalized $\gamma$-ray intensity (Eq. S12) for the absorber at rest (A=0) at constant time $t_c$ as difference of the intensity out of resonance $[I(t_c)_{|\Delta\to\infty} = 1]$ and at the resonance $(I(t_c)_{\Delta=0})$. For this calculation the optical thickness $T_{\rm a} = 7.6$ and the hyperfine magnetic field $B_{\rm hf} = 0.58$ T were used and $a_{\rm n}$ was determined to be 0.786, see Fig. S3(b).

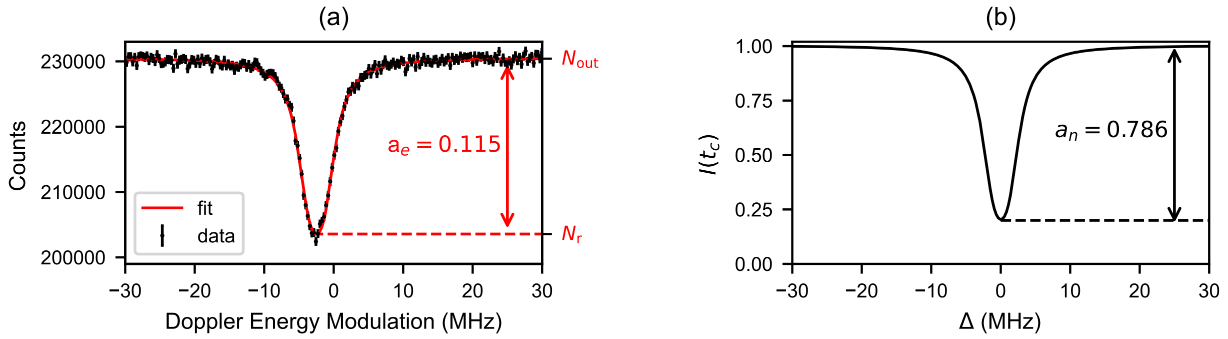


FIG. S3: Determination of: absorption peak amplitude $a_{\rm e}$ from the transmission spectrum (a) and normalized nuclear absorption $a_{\rm n}$ from calculations (b).

The apparatus time resolution, consisting of the single scintillation detector, was determined by fitting the $\gamma$-ray intensity waveforms containing bunches of double and triple pulses. These waveforms were used because the valley depth between the pulses is, unlike the other parameters, highly sensitive to the apparatus time resolution. The bunches were created by absorber sinusoidally vibrating at 10 MHz ($V_{\rm d} = 8V_{\rm pp}$) and tuning the energy of incident radiation between the second and the third sideband ($\Delta = \langle 2f, 3f\rangle$). The apparatus time resolution was determined as an average of four values obtained by fitting the results shown in Fig. S4, and it was $\sigma_{\rm t} = 5.1 \pm 0.3$ ns (12 ns FWHM).

Resulting frequency response function of the piezo transducer was measured at 47 points for 12 frequencies, see Fig. S5. To calculate the voltage waveforms from the frequency response function for realization of the particular motion profiles, the values between the measured points were linearly interpolated. For low driving voltages the amplitude was linearly approximated to zero and phase was kept constant at the value measured for the lowest driving voltage.

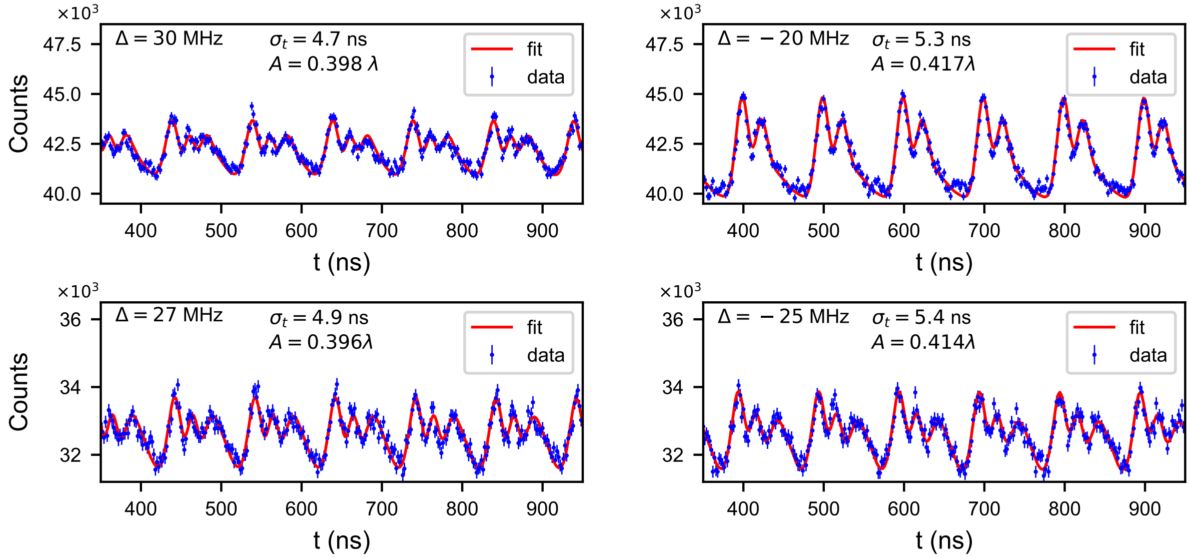


FIG. S4: Determination of apparatus time resolution $\sigma_t$ by fitting $\gamma$-ray intensity waveforms containing double and triple pulses.

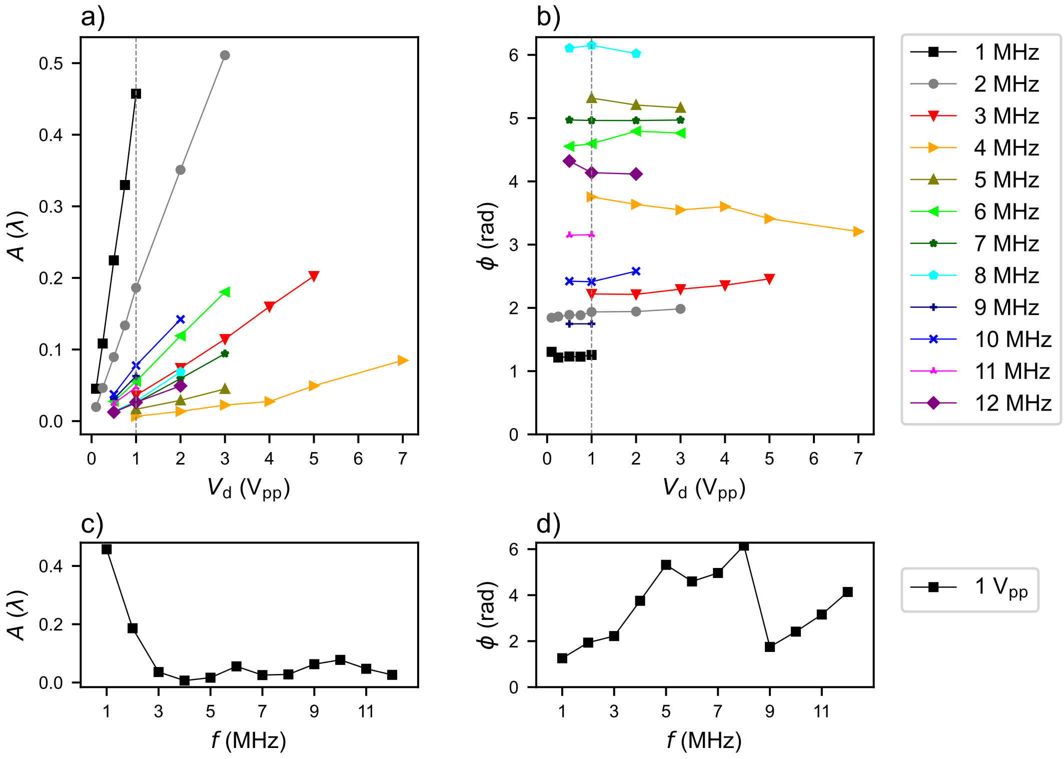


FIG. S5: Measured amplitude (a) and phase (b) response function of the piezo transducer for 12 harmonics and fundamental frequency $f = 1\,\mathrm{MHz}$. Amplitude and phase response for the constant driving voltage $V_\mathrm{d} = 1V_\mathrm{pp}$ are in (c) and (d) respectively. A fast change of phase at 9 MHz is caused by shifting the phase values in the interval $\langle 0, 2\pi \rangle$. The low amplitude response at 4 MHz and 5 MHz was problematic when performing motions with higher amplitudes.

## IV. NORMALIZATION OF EXPERIMENTAL DATA.

To compare the experimental results with simulations, which consider only resonant $\gamma$-photons, the non-resonant background has to be subtracted and the remaining part normalized. The experimentally measured intensity defined by Eq. S13 can be rewritten in the form

$$I_{\exp}(t) = \frac{N}{1 + A_{\mathrm{bcg}}} \left[ I(t) \exp\left( -\frac{t}{C_{\mathrm{b}}} \right) + A_{\mathrm{bcg}} \exp\left( -\frac{t}{C_{\mathrm{b}}} \right) \right] * G(t). \tag{S18}$$

Using the distributivity of convolution and taking into account that $C_{\mathrm{b}} >> \sigma_{\mathrm{t}}$ (in our experiments $C_b \approx 80\,\mu$s), the effect of convolution with Gaussian time resolution on the expression $\exp\left(-t/C_{\mathrm{b}}\right)$ can be neglected, which results in:

$$I_{\exp}(t) = \frac{N}{1 + A_{\mathrm{bcg}}} \left[ I(t) \exp\left( -\frac{t}{C_{\mathrm{b}}} \right) * G(t) + A_{\mathrm{bcg}} \exp\left( -\frac{t}{C_{\mathrm{b}}} \right) \right], \tag{S19}$$

where the expression

$$I(t) \exp\left( -\frac{t}{C_{\mathrm{b}}} \right) * G(t) = I/I_0, \tag{S20}$$

describes the intensity normalized to the incident $\gamma$-ray intensity of resonant photons, including the apparatus effects, primarily the time resolution. Factoring this expression out then gives the formula

$$I/I_0 = \frac{I_{\exp}(t)\,(1 + A_{\mathrm{bcg}})}{N} - A_{\mathrm{bcg}} \exp\left( -\frac{t}{C_{\mathrm{b}}} \right), \tag{S21}$$

which was applied to get the normalized experimental data displayed in Fig. 3 and Fig. 4 in the main paper.
